# Supplementary material for: ScoNe: Benchmarking Negation Reasoning in Language Models With Fine-Tuning and In-Context Learning
Source: arXiv:2305.19426 source file (2023-05-30)
Supplement: Supplementary file 1 [file supp-incontext-results.tex]

\section{Full In-context Learning Results}

\subsection{Conditional Question Prompt}

\promptExample{Is it true that if we didn't eat pizza, then we didn't eat food?}

\subsubsection{text-davinci-002}

\begin{center}
\begin{tabular}{lrrr}
\toprule
{} &  Incorrect &  Correct &  Accuracy \\
\midrule
both\_not\_scope    &         70 &      130 &      0.65 \\
double\_neg        &         99 &      101 &      0.51 \\
not\_scoped        &         91 &      109 &      0.55 \\
one\_scope\_one\_not &        100 &      100 &      0.50 \\
All               &        360 &      440 &      0.55 \\
\bottomrule
\end{tabular}
\end{center}

\subsubsection{text-davinci-003}

\begin{center}
\begin{tabular}{lrrr}
\toprule
{} &  Incorrect &  Correct &  Accuracy \\
\midrule
both\_not\_scope    &         37 &      163 &      0.81 \\
double\_neg        &        100 &      100 &      0.50 \\
not\_scoped        &         30 &      170 &      0.85 \\
one\_scope\_one\_not &        112 &       88 &      0.44 \\
All               &        279 &      521 &      0.65 \\
\bottomrule
\end{tabular}
\end{center}

\subsection{Few-Shot Conditional Question Prompt}

\promptExample{Q1: Is it true that if a not so tall person reading a paper is not currently sitting inside a building, then a not so tall person reading a paper is not currently sitting inside a diner?\mynewline
A1: Yes\mynewline
\mynewline
Q2: Is it true that if a not so tall person reading a paper is not currently sitting inside a building, then a not so tall person reading a paper is not currently sitting inside a court?\mynewline
A2: Yes\mynewline
\mynewline
Q3: Is it true that if a not so tall person reading a paper is not currently sitting inside a opera, then a not so tall person reading a paper is not currently sitting inside a building?\mynewline
A3: Maybe\mynewline

Q4: Is it true that if the girl will not get a stuffed pinscher as a gift, but not because she failed the exam, then the girl will not get a stuffed dog as a gift, but not because she failed the exam?
A4: Maybe

Q: Is it true that if we didn't eat pizza, then we didn't eat food?
A:}

\subsubsection{text-davinci-002}

\begin{center}
\begin{tabular}{lrrr}
\toprule
{} &  Incorrect &  Correct &  Accuracy \\
\midrule
both\_not\_scope    &         43 &      157 &      0.79 \\
double\_neg        &         97 &      103 &      0.52 \\
not\_scoped        &         37 &      163 &      0.81 \\
one\_scope\_one\_not &        135 &       65 &      0.33 \\
All               &        312 &      488 &      0.61 \\
\bottomrule
\end{tabular}
\end{center}

\subsubsection{text-davinci-003}

\begin{center}
\begin{tabular}{lrrr}
\toprule
{} &  Incorrect &  Correct &  Accuracy \\
\midrule
both\_not\_scope    &         22 &      178 &      0.89 \\
double\_neg        &         84 &      116 &      0.58 \\
not\_scoped        &         36 &      164 &      0.82 \\
one\_scope\_one\_not &        138 &       62 &      0.31 \\
All               &        280 &      520 &      0.65 \\
\bottomrule
\end{tabular}
\end{center}

\subsection{Hypothesis Question Prompt}

\promptExample{Assume that we didn't eat pizza. Is it then definitely true that we didn't eat food? Answer Yes or No.}

\subsubsection{text-davinci-002}

\begin{center}
\begin{tabular}{lrrr}
\toprule
{} &  Incorrect &  Correct &  Accuracy \\
\midrule
both\_not\_scope    &         28 &      172 &      0.86 \\
double\_neg        &         75 &      125 &      0.62 \\
not\_scoped        &         34 &      166 &      0.83 \\
one\_scope\_one\_not &        120 &       80 &      0.40 \\
All               &        257 &      543 &      0.68 \\
\bottomrule
\end{tabular}
\end{center}

\subsubsection{text-davinci-003}

\begin{center}
\begin{tabular}{lrrr}
\toprule
{} &  Incorrect &  Correct &  Accuracy \\
\midrule
both\_not\_scope    &         59 &      141 &      0.70 \\
double\_neg        &         98 &      102 &      0.51 \\
not\_scoped        &         20 &      180 &      0.90 \\
one\_scope\_one\_not &        116 &       84 &      0.42 \\
All               &        293 &      507 &      0.63 \\
\bottomrule
\end{tabular}
\end{center}

\subsection{Few-Shot Hypothesis Question Prompt}

\promptExample{Q1: Assume that the man does not own a dog and does not own a cat. Is it then definitely true that the man does not own a sheepdog and does not own a cat? Answer Yes or No.\mynewline
A1: Yes\mynewline
\mynewline
Q2: Assume that a not so tall person reading a paper is not currently sitting inside a building. Is it then definitely true that a not so tall person reading a paper is not currently sitting inside a school? Answer Yes or No.\mynewline
A2: Yes\mynewline
\mynewline
Q3: Assume that the man does not own a hound and does not own a cat. Is it then definitely true that the man does not own a dog and does not own a cat? Answer Yes or No.\mynewline
A3: No\mynewline

Q4: Assume that the man does not own a doberman and does not own a cat. Is it then definitely true that the man does not own a dog and does not own a cat? Answer Yes or No.
A4: No

Q: Assume that we didn't eat pizza. Is it then definitely true that we didn't eat food? Answer Yes or No.
A:}

\subsubsection{text-davinci-002}

\begin{center}
\begin{tabular}{lrrr}
\toprule
{} &  Incorrect &  Correct &  Accuracy \\
\midrule
both\_not\_scope    &         15 &      185 &      0.93 \\
double\_neg        &         63 &      137 &      0.69 \\
not\_scoped        &         18 &      182 &      0.91 \\
one\_scope\_one\_not &        120 &       80 &      0.40 \\
All               &        216 &      584 &      0.73 \\
\bottomrule
\end{tabular}
\end{center}

\subsubsection{text-davinci-003}

\begin{center}
\begin{tabular}{lrrr}
\toprule
{} &  Incorrect &  Correct &  Accuracy \\
\midrule
both\_not\_scope    &          9 &      191 &      0.95 \\
double\_neg        &         35 &      165 &      0.82 \\
not\_scoped        &          6 &      194 &      0.97 \\
one\_scope\_one\_not &        117 &       83 &      0.41 \\
All               &        167 &      633 &      0.79 \\
\bottomrule
\end{tabular}
\end{center}

\subsection{Conditional Truth Evaluation Prompt}

\promptExample{If we didn't eat pizza, then we didn't eat food. Is this true?}

\subsubsection{text-davinci-002}

\begin{center}
\begin{tabular}{lrrr}
\toprule
{} &  Incorrect &  Correct &  Accuracy \\
\midrule
both\_not\_scope    &         69 &      131 &      0.66 \\
double\_neg        &         80 &      120 &      0.60 \\
not\_scoped        &         72 &      128 &      0.64 \\
one\_scope\_one\_not &         86 &      114 &      0.57 \\
All               &        307 &      493 &      0.62 \\
\bottomrule
\end{tabular}
\end{center}

\subsubsection{text-davinci-003}

\begin{center}
\begin{tabular}{lrrr}
\toprule
{} &  Incorrect &  Correct &  Accuracy \\
\midrule
both\_not\_scope    &         39 &      161 &      0.81 \\
double\_neg        &        113 &       87 &      0.43 \\
not\_scoped        &         28 &      172 &      0.86 \\
one\_scope\_one\_not &        104 &       96 &      0.48 \\
All               &        284 &      516 &      0.65 \\
\bottomrule
\end{tabular}
\end{center}

\subsection{Few-Shot Conditional Truth Evaluation Prompt}

\promptExample{C1: If the girl will not get a stuffed dog as a gift, but not because she failed the exam, then the girl will not get a stuffed bulldog as a gift, but not because she failed the exam. Is this true?\mynewline
A1: Yes\mynewline
\mynewline
C2: If the man does not own a mammal and does not own a cat, then the man does not own a dog and does not own a cat. Is this true?\mynewline
A2: Yes\mynewline
\mynewline
C3: If the man, who's eyes are not open, is not steering a sedan, then the man, who's eyes are not open, is not steering a car. Is this true?\mynewline
A3: Maybe\mynewline

C4: If the girl will not get a stuffed dog as a gift, but not because she failed the exam, then the girl will not get a stuffed mammal as a gift, but not because she failed the exam. Is this true?
A4: Maybe

C:If we didn't eat pizza, then we didn't eat food. Is this true?
A:}

\subsubsection{text-davinci-002}

\begin{center}
\begin{tabular}{lrrr}
\toprule
{} &  Incorrect &  Correct &  Accuracy \\
\midrule
both\_not\_scope    &         23 &      177 &      0.89 \\
double\_neg        &         82 &      118 &      0.59 \\
not\_scoped        &         22 &      178 &      0.89 \\
one\_scope\_one\_not &        126 &       74 &      0.37 \\
All               &        253 &      547 &      0.68 \\
\bottomrule
\end{tabular}
\end{center}

\subsubsection{text-davinci-003}

\begin{center}
\begin{tabular}{lrrr}
\toprule
{} &  Incorrect &  Correct &  Accuracy \\
\midrule
both\_not\_scope    &         18 &      182 &      0.91 \\
double\_neg        &         71 &      129 &      0.65 \\
not\_scoped        &         17 &      183 &      0.92 \\
one\_scope\_one\_not &        131 &       69 &      0.34 \\
All               &        237 &      563 &      0.70 \\
\bottomrule
\end{tabular}
\end{center}

\subsection{Brown Et Al Style Prompt}

\promptExample{C: We didn't eat pizza\mynewline
Q: We didn't eat food. Yes, No, or Maybe?}

\subsubsection{text-davinci-002}

\begin{center}
\begin{tabular}{lrrr}
\toprule
{} &  Incorrect &  Correct &  Accuracy \\
\midrule
both\_not\_scope    &         82 &      118 &      0.59 \\
double\_neg        &         90 &      110 &      0.55 \\
not\_scoped        &         81 &      119 &      0.59 \\
one\_scope\_one\_not &        103 &       97 &      0.48 \\
All               &        356 &      444 &      0.56 \\
\bottomrule
\end{tabular}
\end{center}

\subsubsection{text-davinci-003}

\begin{center}
\begin{tabular}{lrrr}
\toprule
{} &  Incorrect &  Correct &  Accuracy \\
\midrule
both\_not\_scope    &         52 &      148 &      0.74 \\
double\_neg        &         92 &      108 &      0.54 \\
not\_scoped        &         60 &      140 &      0.70 \\
one\_scope\_one\_not &        112 &       88 &      0.44 \\
All               &        316 &      484 &      0.60 \\
\bottomrule
\end{tabular}
\end{center}

\subsection{Few-Shot Brown Et Al Style Prompt}

\promptExample{C1: the man does not own a dog and does not own a cat.\mynewline
Q1: the man does not own a schnauzer and does not own a cat. Yes, No, or Maybe?\mynewline
A2: Yes\mynewline
\mynewline
C2: The girl will not get a stuffed dog as a gift, but not because she failed the exam.\mynewline
Q2: The girl will not get a stuffed dachshund as a gift, but not because she failed the exam. Yes, No, or Maybe?\mynewline
A3: Yes\mynewline
\mynewline
C3: A not so tall person reading a paper is not currently sitting inside a skyscraper.
Q3: A not so tall person reading a paper is not currently sitting inside a building. Yes, No, or Maybe?
A4: Maybe

C4: A not so tall person reading a paper is not currently sitting inside a monastery.
Q4: A not so tall person reading a paper is not currently sitting inside a building. Yes, No, or Maybe?
A5: Maybe

C: We didn't eat pizza
Q: We didn't eat food. Yes, No, or Maybe?
A:}

\subsubsection{text-davinci-002}

\begin{center}
\begin{tabular}{lrrr}
\toprule
{} &  Incorrect &  Correct &  Accuracy \\
\midrule
both\_not\_scope    &         43 &      157 &      0.79 \\
double\_neg        &         57 &      143 &      0.71 \\
not\_scoped        &         50 &      150 &      0.75 \\
one\_scope\_one\_not &        142 &       58 &      0.29 \\
All               &        292 &      508 &      0.64 \\
\bottomrule
\end{tabular}
\end{center}

\subsubsection{text-davinci-003}

\begin{center}
\begin{tabular}{lrrr}
\toprule
{} &  Incorrect &  Correct &  Accuracy \\
\midrule
both\_not\_scope    &         46 &      154 &      0.77 \\
double\_neg        &         31 &      169 &      0.84 \\
not\_scoped        &         82 &      118 &      0.59 \\
one\_scope\_one\_not &        138 &       62 &      0.31 \\
All               &        297 &      503 &      0.63 \\
\bottomrule
\end{tabular}
\end{center}

\subsection{Structured Prompt}

\promptExample{P: We didn't eat pizza\mynewline
H: We didn't eat food\mynewline
L:}

\subsubsection{text-davinci-002}

\begin{center}
\begin{tabular}{lrrr}
\toprule
{} &  Incorrect &  Correct &  Accuracy \\
\midrule
both\_not\_scope    &        100 &      100 &      0.50 \\
double\_neg        &        100 &      100 &      0.50 \\
not\_scoped        &        100 &      100 &      0.50 \\
one\_scope\_one\_not &        100 &      100 &      0.50 \\
All               &        400 &      400 &      0.50 \\
\bottomrule
\end{tabular}
\end{center}

\subsubsection{text-davinci-003}

\begin{center}
\begin{tabular}{lrrr}
\toprule
{} &  Incorrect &  Correct &  Accuracy \\
\midrule
both\_not\_scope    &        100 &      100 &      0.50 \\
double\_neg        &        100 &      100 &      0.50 \\
not\_scoped        &        100 &      100 &      0.50 \\
one\_scope\_one\_not &        100 &      100 &      0.50 \\
All               &        400 &      400 &      0.50 \\
\bottomrule
\end{tabular}
\end{center}

\subsection{Few-Shot Structured Prompt}

\promptExample{P1: A not so tall person reading a paper is not currently sitting inside a building.\mynewline
H1: A not so tall person reading a paper is not currently sitting inside a manor.\mynewline
L1: entailment\mynewline
\mynewline
P2: A dog not on the playground did not catch any ball.\mynewline
H2: A dog not on the playground did not catch any softball.\mynewline
L2: entailment\mynewline
\mynewline
P3: The girl will not get a stuffed schnauzer as a gift, but not because she failed the exam.
H3: The girl will not get a stuffed dog as a gift, but not because she failed the exam.
L3: neutral

P4: A not so tall person reading a paper is not currently sitting inside a pub.
H4: A not so tall person reading a paper is not currently sitting inside a building.
L4: neutral

P: We didn't eat pizza
H: We didn't eat food
L:}

\subsubsection{text-davinci-002}

\begin{center}
\begin{tabular}{lrrr}
\toprule
{} &  Incorrect &  Correct &  Accuracy \\
\midrule
both\_not\_scope    &        100 &      100 &      0.50 \\
double\_neg        &        100 &      100 &      0.50 \\
not\_scoped        &        100 &      100 &      0.50 \\
one\_scope\_one\_not &        100 &      100 &      0.50 \\
All               &        400 &      400 &      0.50 \\
\bottomrule
\end{tabular}
\end{center}

\subsubsection{text-davinci-003}

\begin{center}
\begin{tabular}{lrrr}
\toprule
{} &  Incorrect &  Correct &  Accuracy \\
\midrule
both\_not\_scope    &        100 &      100 &      0.50 \\
double\_neg        &        100 &      100 &      0.50 \\
not\_scoped        &        100 &      100 &      0.50 \\
one\_scope\_one\_not &        100 &      100 &      0.50 \\
All               &        400 &      400 &      0.50 \\
\bottomrule
\end{tabular}
\end{center}

\subsection{Reasoning Prompt}

\promptExample{Logical and commonsense reasoning exam.\mynewline
\mynewline
Explain your reasoning in detail, then answer with Yes or No. Your answers should follow this 4-line format:\mynewline
\mynewline
Premise: <a tricky logical statement about the world>.\mynewline
Question: <question requiring logical deduction>.\mynewline
Reasoning: <an explanation of what you understand about the possible scenarios>.\mynewline
Answer: <Yes or No>.\mynewline

Premise: we didn't eat pizza
Question: Can we logically conclude for sure that we didn't eat food?
Reasoning: Let's think logically step by step. The premise basically tells us that}

\subsubsection{text-davinci-002}

\begin{center}
\begin{tabular}{lrrr}
\toprule
{} &  Incorrect &  Correct &  Accuracy \\
\midrule
both\_not\_scope    &         63 &      137 &      0.69 \\
double\_neg        &         77 &      123 &      0.61 \\
not\_scoped        &         61 &      139 &      0.69 \\
one\_scope\_one\_not &         87 &      113 &      0.56 \\
All               &        288 &      512 &      0.64 \\
\bottomrule
\end{tabular}
\end{center}

\subsubsection{text-davinci-003}

\begin{center}
\begin{tabular}{lrrr}
\toprule
{} &  Incorrect &  Correct &  Accuracy \\
\midrule
both\_not\_scope    &         14 &      186 &      0.93 \\
double\_neg        &         57 &      143 &      0.71 \\
not\_scoped        &         24 &      176 &      0.88 \\
one\_scope\_one\_not &        107 &       93 &      0.47 \\
All               &        202 &      598 &      0.75 \\
\bottomrule
\end{tabular}
\end{center}
